# Supplementary material for: A Geometric Framework for Adversarial Vulnerability in Machine Learning
Source: arXiv:2407.11029 source file (2024-07-03)
Supplement: Supplementary file 1 [file AppendixA.tex]

% % Appendix A

% \chapter{Frequently Asked Questions} % Main appendix title; replace with name of appendix
% \label{AppendixA} % For referencing this appendix elsewhere, use \ref{AppendixA}


% \section{How do I change the colors of links?}

% The color of links can be changed to your liking using:

% {\small\verb!\hypersetup{urlcolor=red}!}, or

% {\small\verb!\hypersetup{citecolor=green}!}, or

% {\small\verb!\hypersetup{allcolor=blue}!}.

% \noindent If you want to completely hide the links, you can use:

% {\small\verb!\hypersetup{allcolors=.}!}, or even better: 

% {\small\verb!\hypersetup{hidelinks}!}.

% {\small\verb!\hypersetup{colorlinks=false}!}.

% \section{Getting Started with this Template}

% If you are familiar with \LaTeX{}, then you should explore the directory structure of the template and then proceed to place your own information into the \emph{THESIS INFORMATION} block of the \file{Dissertation.tex} file. You can then modify the rest of this file to your unique specifications based on your degree/university. Section \ref{FillingFile} on page \pageref{FillingFile} will help you do this. Make sure you also read section \ref{ThesisConventions} about thesis conventions to get the most out of this template.

% If you are new to \LaTeX{} it is recommended that you carry on reading through the rest of the information in this document.

% Before you begin using this template you should ensure that its style complies with the thesis style guidelines imposed by your institution. In most cases this template style and layout will be suitable. If it is not, it may only require a small change to bring the template in line with your institution's recommendations. These modifications will need to be done on the \file{DoctoralThesis.cls} file.

% \subsection{About this Template}

% This \LaTeX{} Thesis Template is originally based and created around a \LaTeX{} style file created by Steve R.\ Gunn from the University of Southampton (UK), department of Electronics and Computer Science. You can find his original thesis style file at his site, here:
% \url{http://www.ecs.soton.ac.uk/~srg/softwaretools/document/templates/}

% Steve's \file{ecsthesis.cls} was then taken by Sunil Patel who modified it by creating a skeleton framework and folder structure to place the thesis files in. The resulting template can be found on Sunil's site here:
% \url{http://www.sunilpatel.co.uk/thesis-template}

% Sunil's template was made available through \url{http://www.LaTeXTemplates.com} where it was modified many times based on user requests and questions. Version 2.0 and onwards of this template represents a major modification to Sunil's template and is, in fact, hardly recognisable. The work to make version 2.0 possible was carried out by \href{mailto:vel@latextemplates.com}{Vel} and Johannes Böttcher.
