# Supplementary material for: A Geometric Framework for Adversarial Vulnerability in Machine Learning
Source: arXiv:2407.11029 source file (2024-07-03)
Supplement: Supplementary file 2 [file AppendixTemplate.tex]

% Appendix Template

\chapter{Type the name of your appendix here} % Main appendix title

\label{AppendixX} % Change X to a consecutive letter; for referencing this appendix elsewhere, use \ref{AppendixX}

Write your Appendix content here.
